# Supplementary material for: Recursive random binning to detect and display pairwise dependence
Source: arXiv:2311.08561 source file (2025-04-29)
Supplement: Supplementary file 1 [file Appendix_dependence_patterns.tex]

\section{Dependence for different patterns}
\label{sec:function}

Take, for example, the dependence patterns displayed in Figure \ref{fig:plotNoiseExample}(a).
\begin{figure}[!ht]
\begin{center}
  \noindent
	\begin{subfigure}[c]{0.5\textwidth}
			\includegraphics[height = 0.5\textheight]{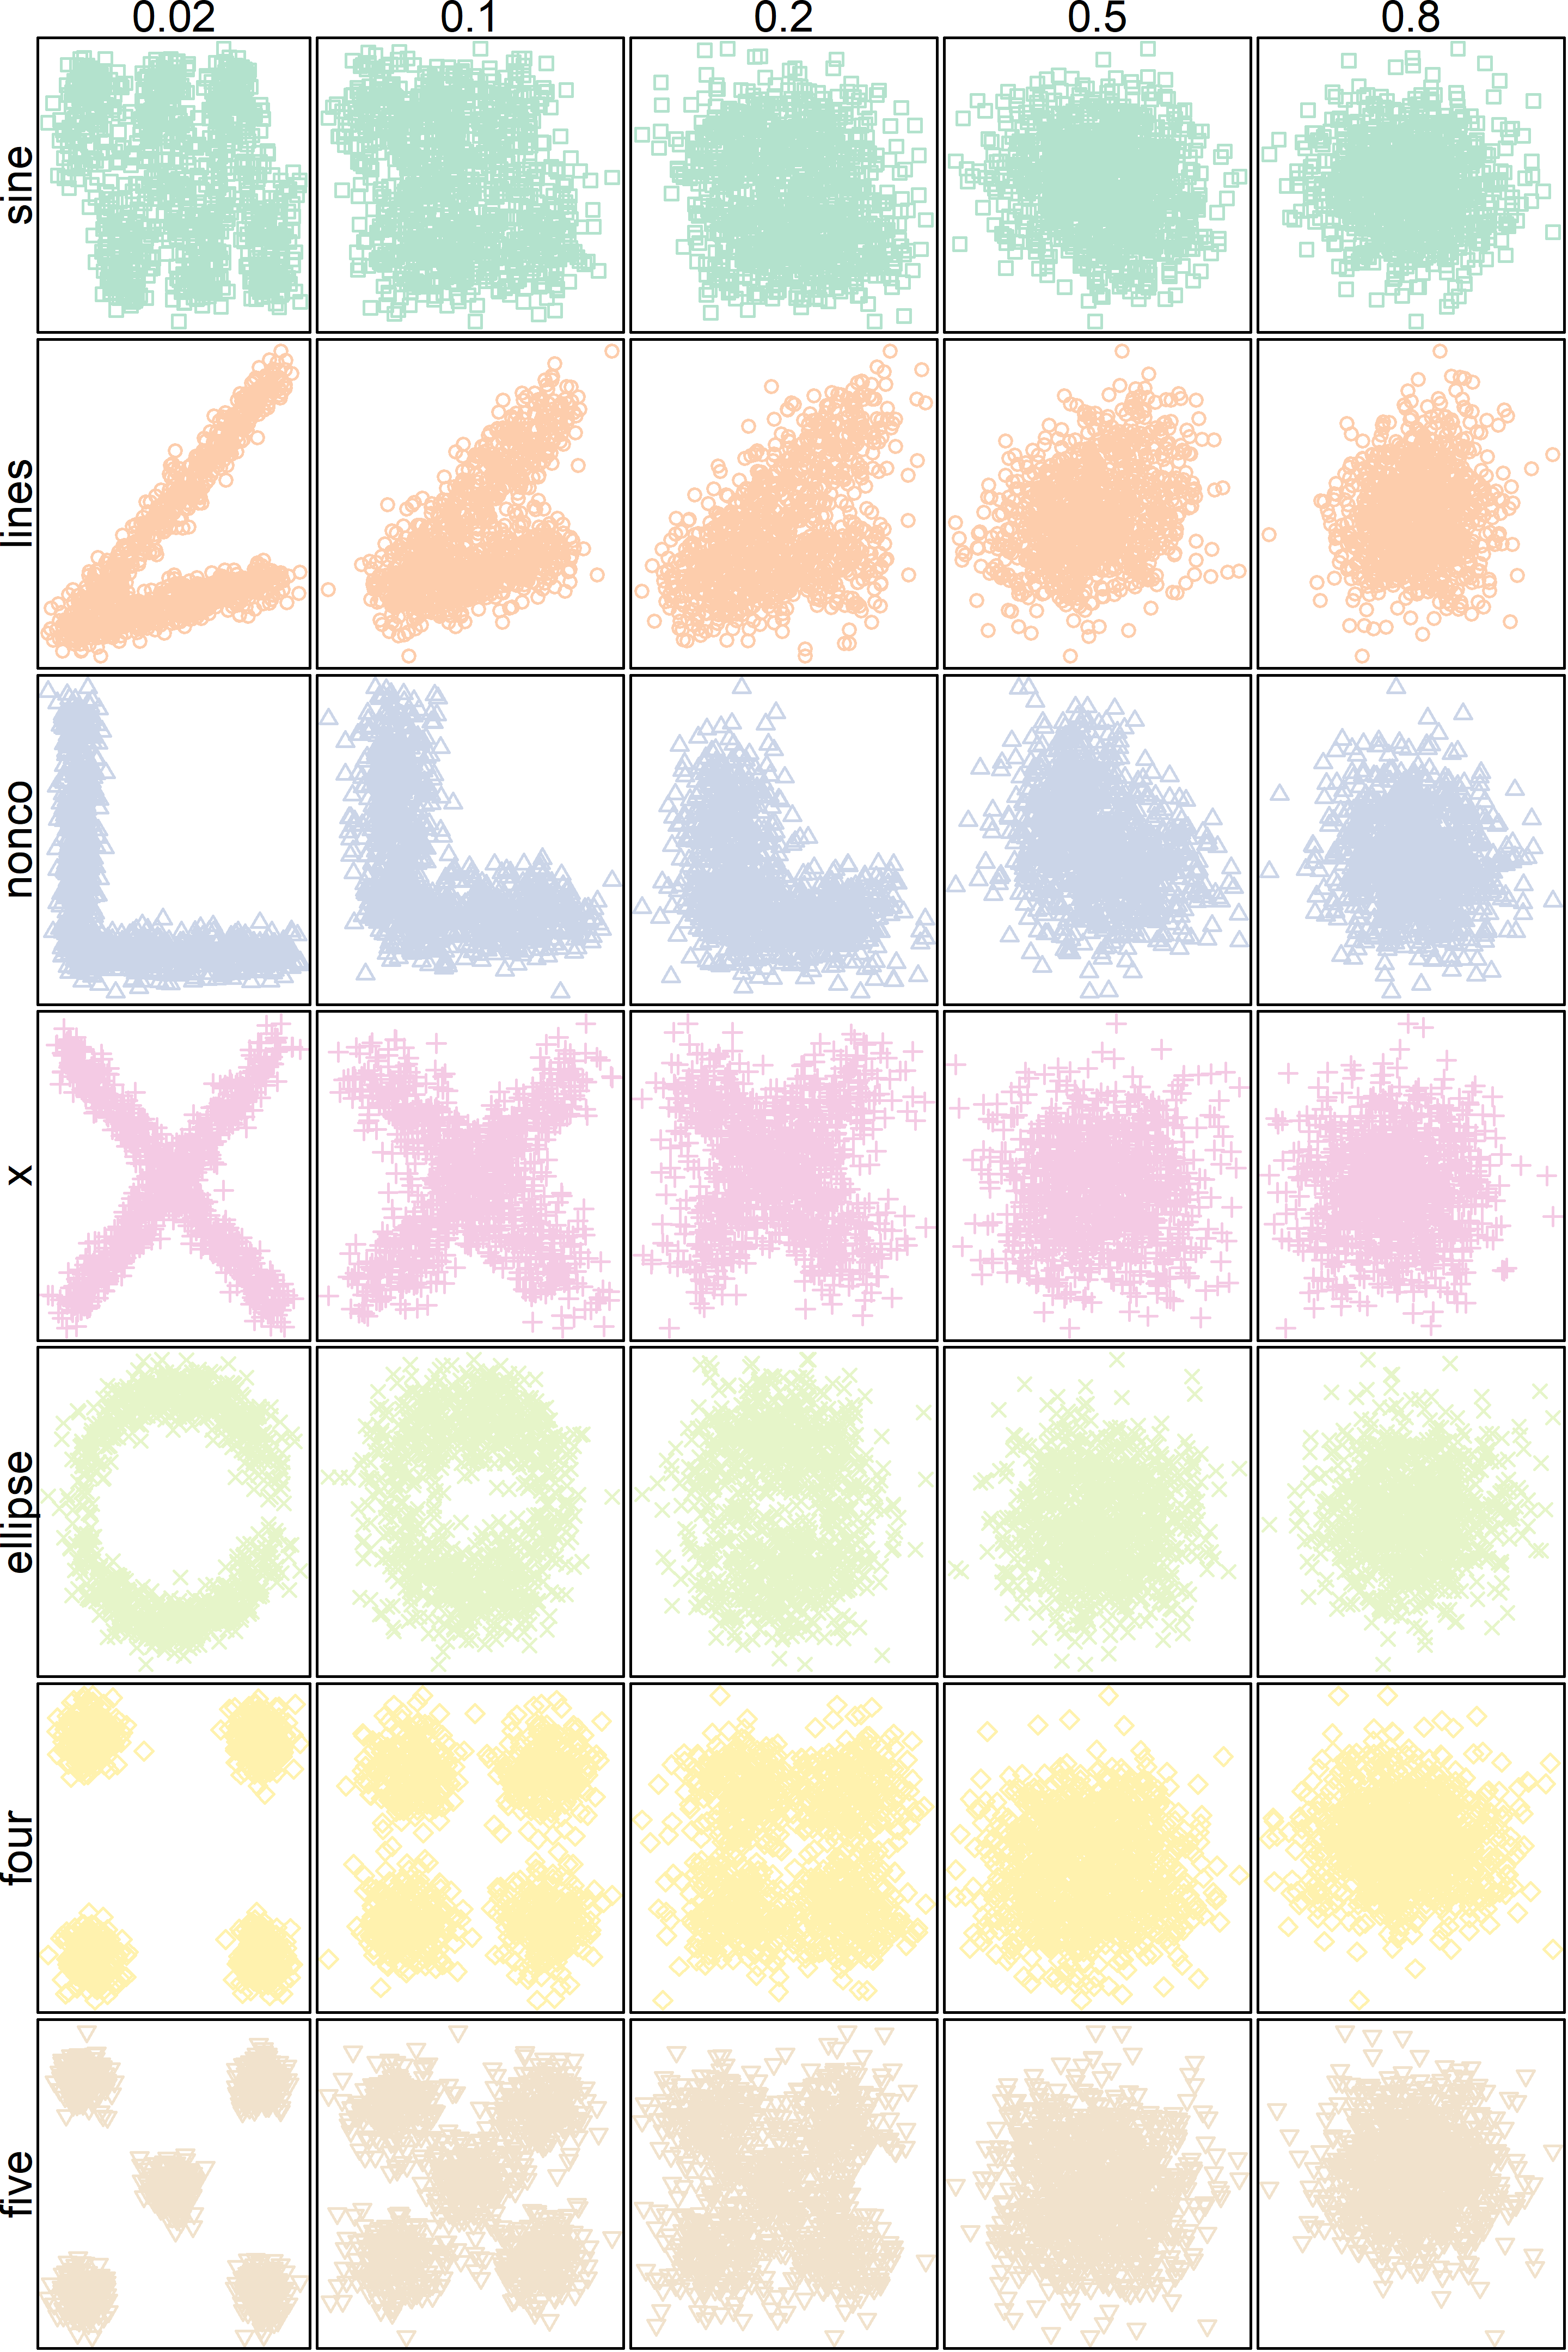} 
	\caption{Raw data patterns by noise level in $y$ }
	\label{fig:plotNoiseExamplePattern}
	\end{subfigure}
        \vspace{-0.1\textheight}
	\begin{tabular}{c}
	\begin{subfigure}[t]{0.4\textwidth}
			\includegraphics[width = \textwidth]{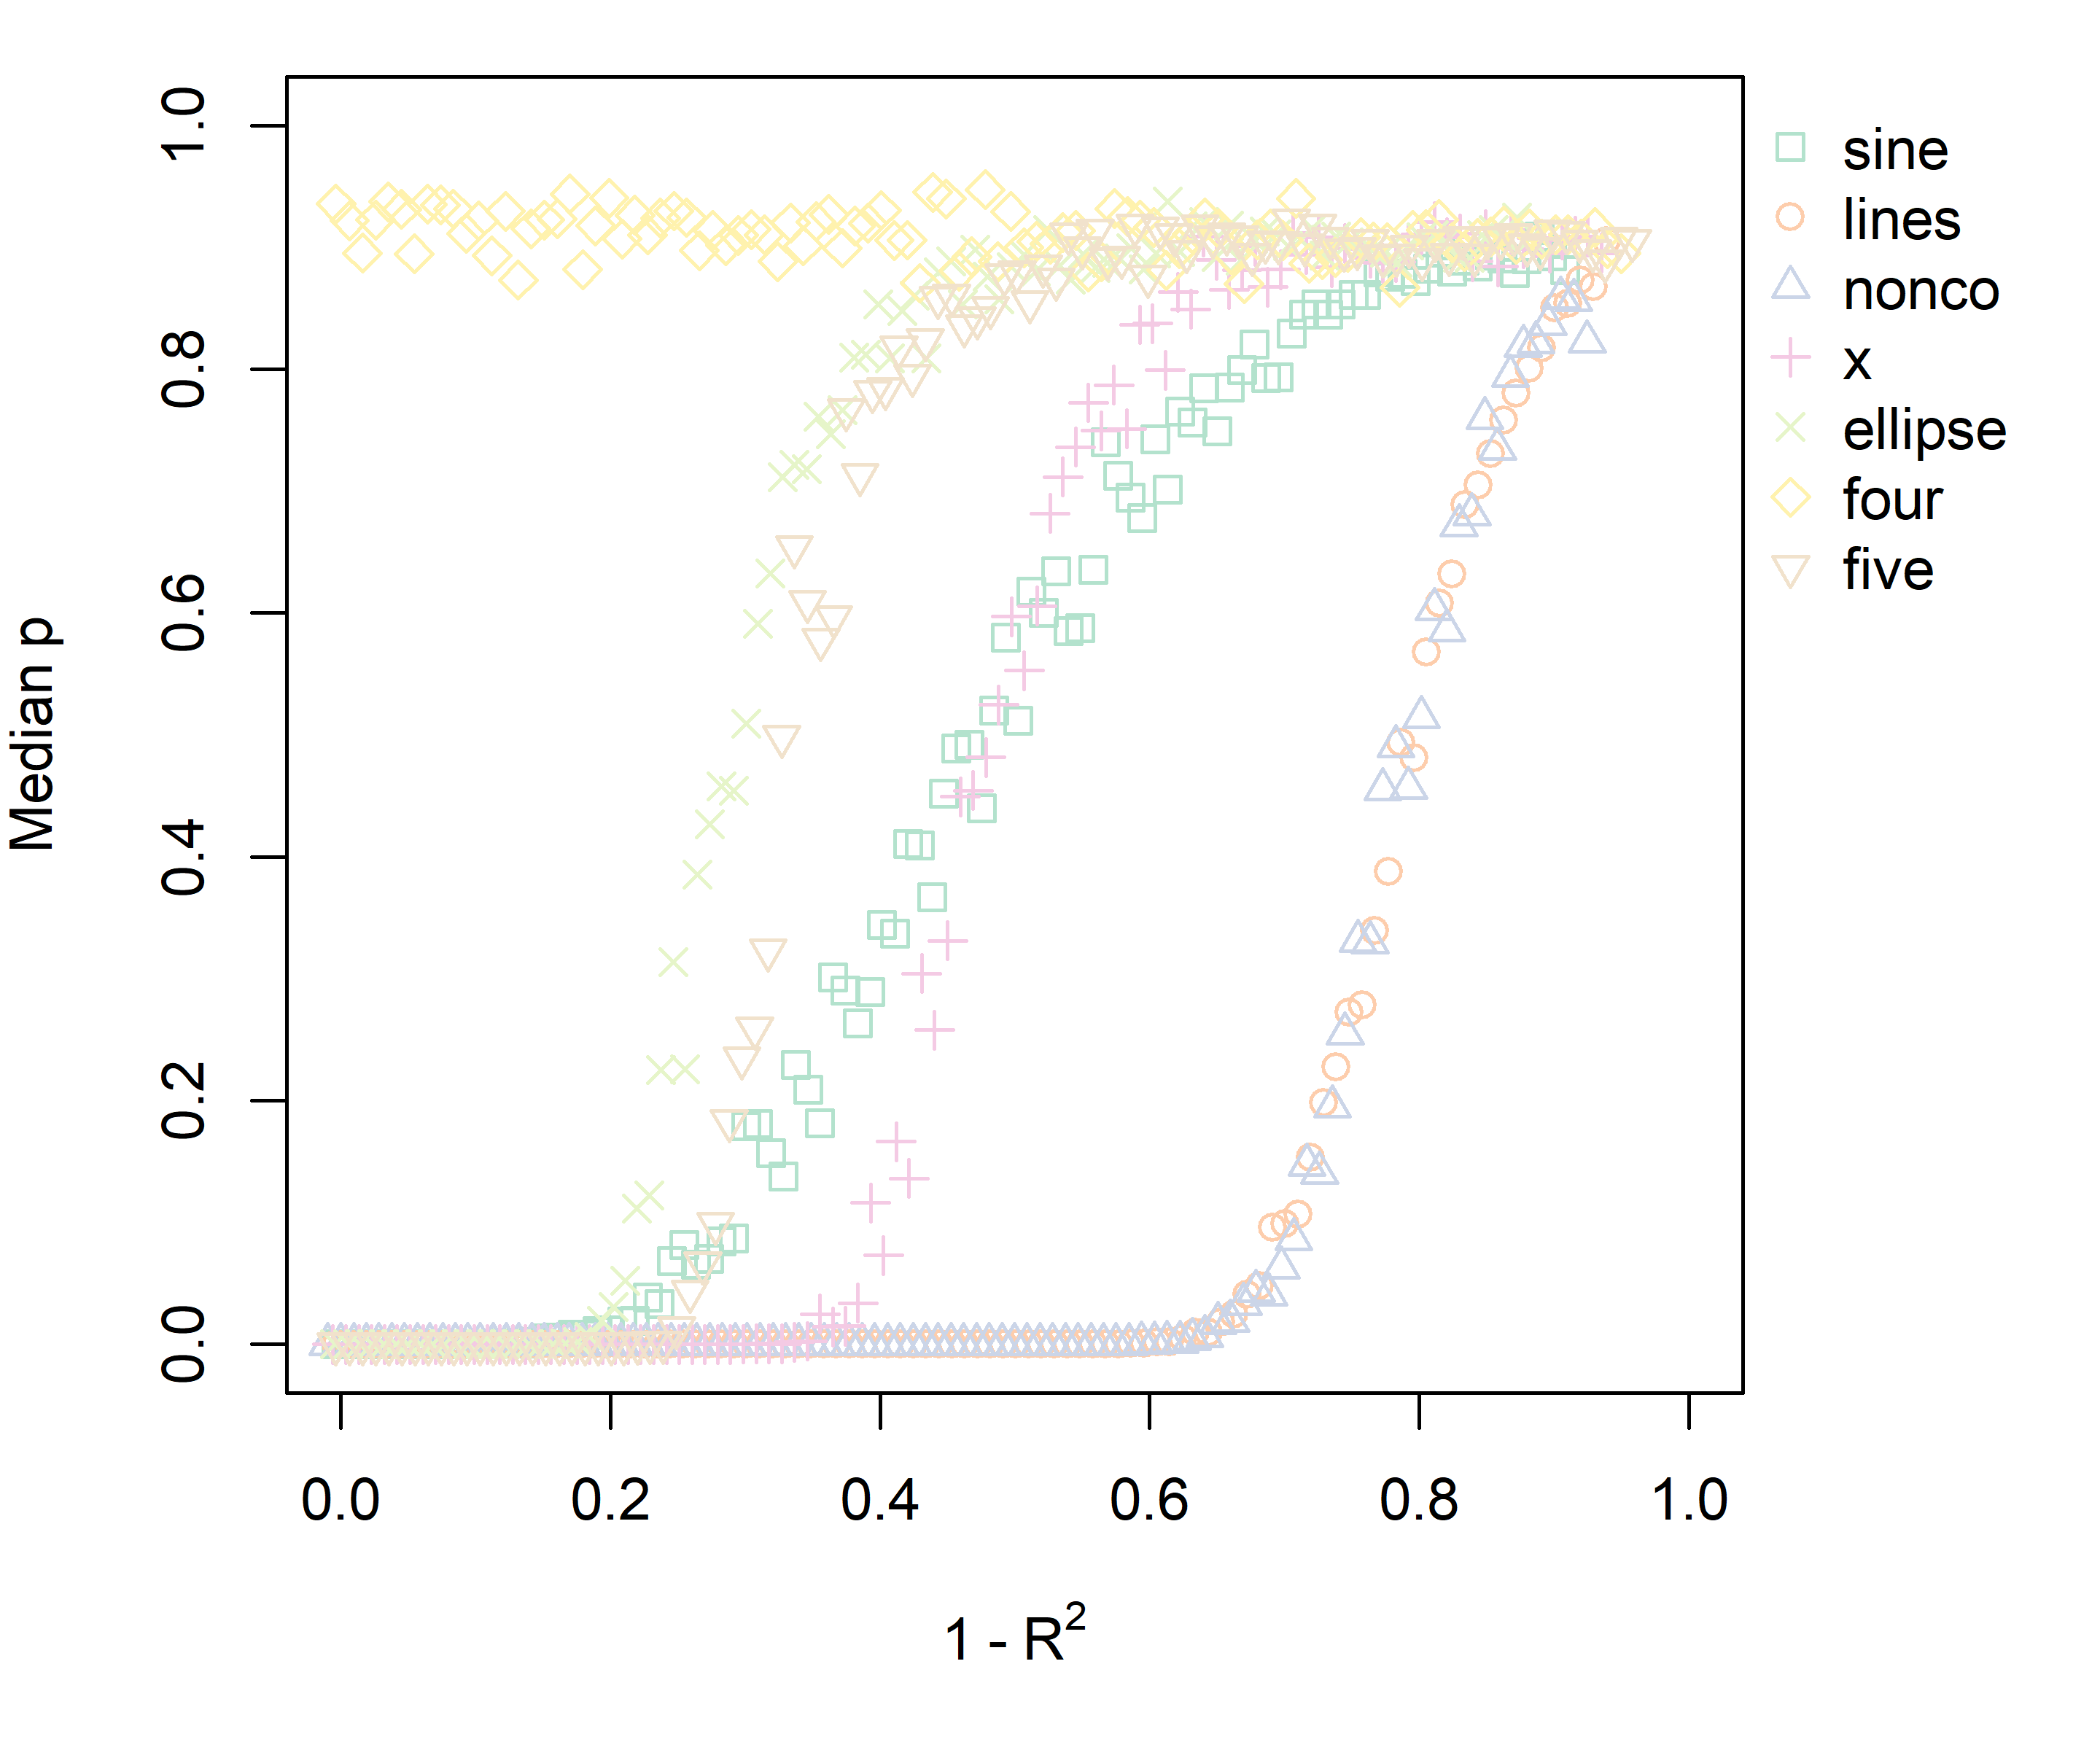} 
			\vspace{-0.04\textheight}
	\caption{\footnotesize Median $p$-value by noise levels}
			\vspace{0.02\textheight}
	\label{fig:plotNoiseExamplePerf}
	\end{subfigure} \\
	\begin{subfigure}[b]{0.4\textwidth}
			\includegraphics[width = \textwidth]{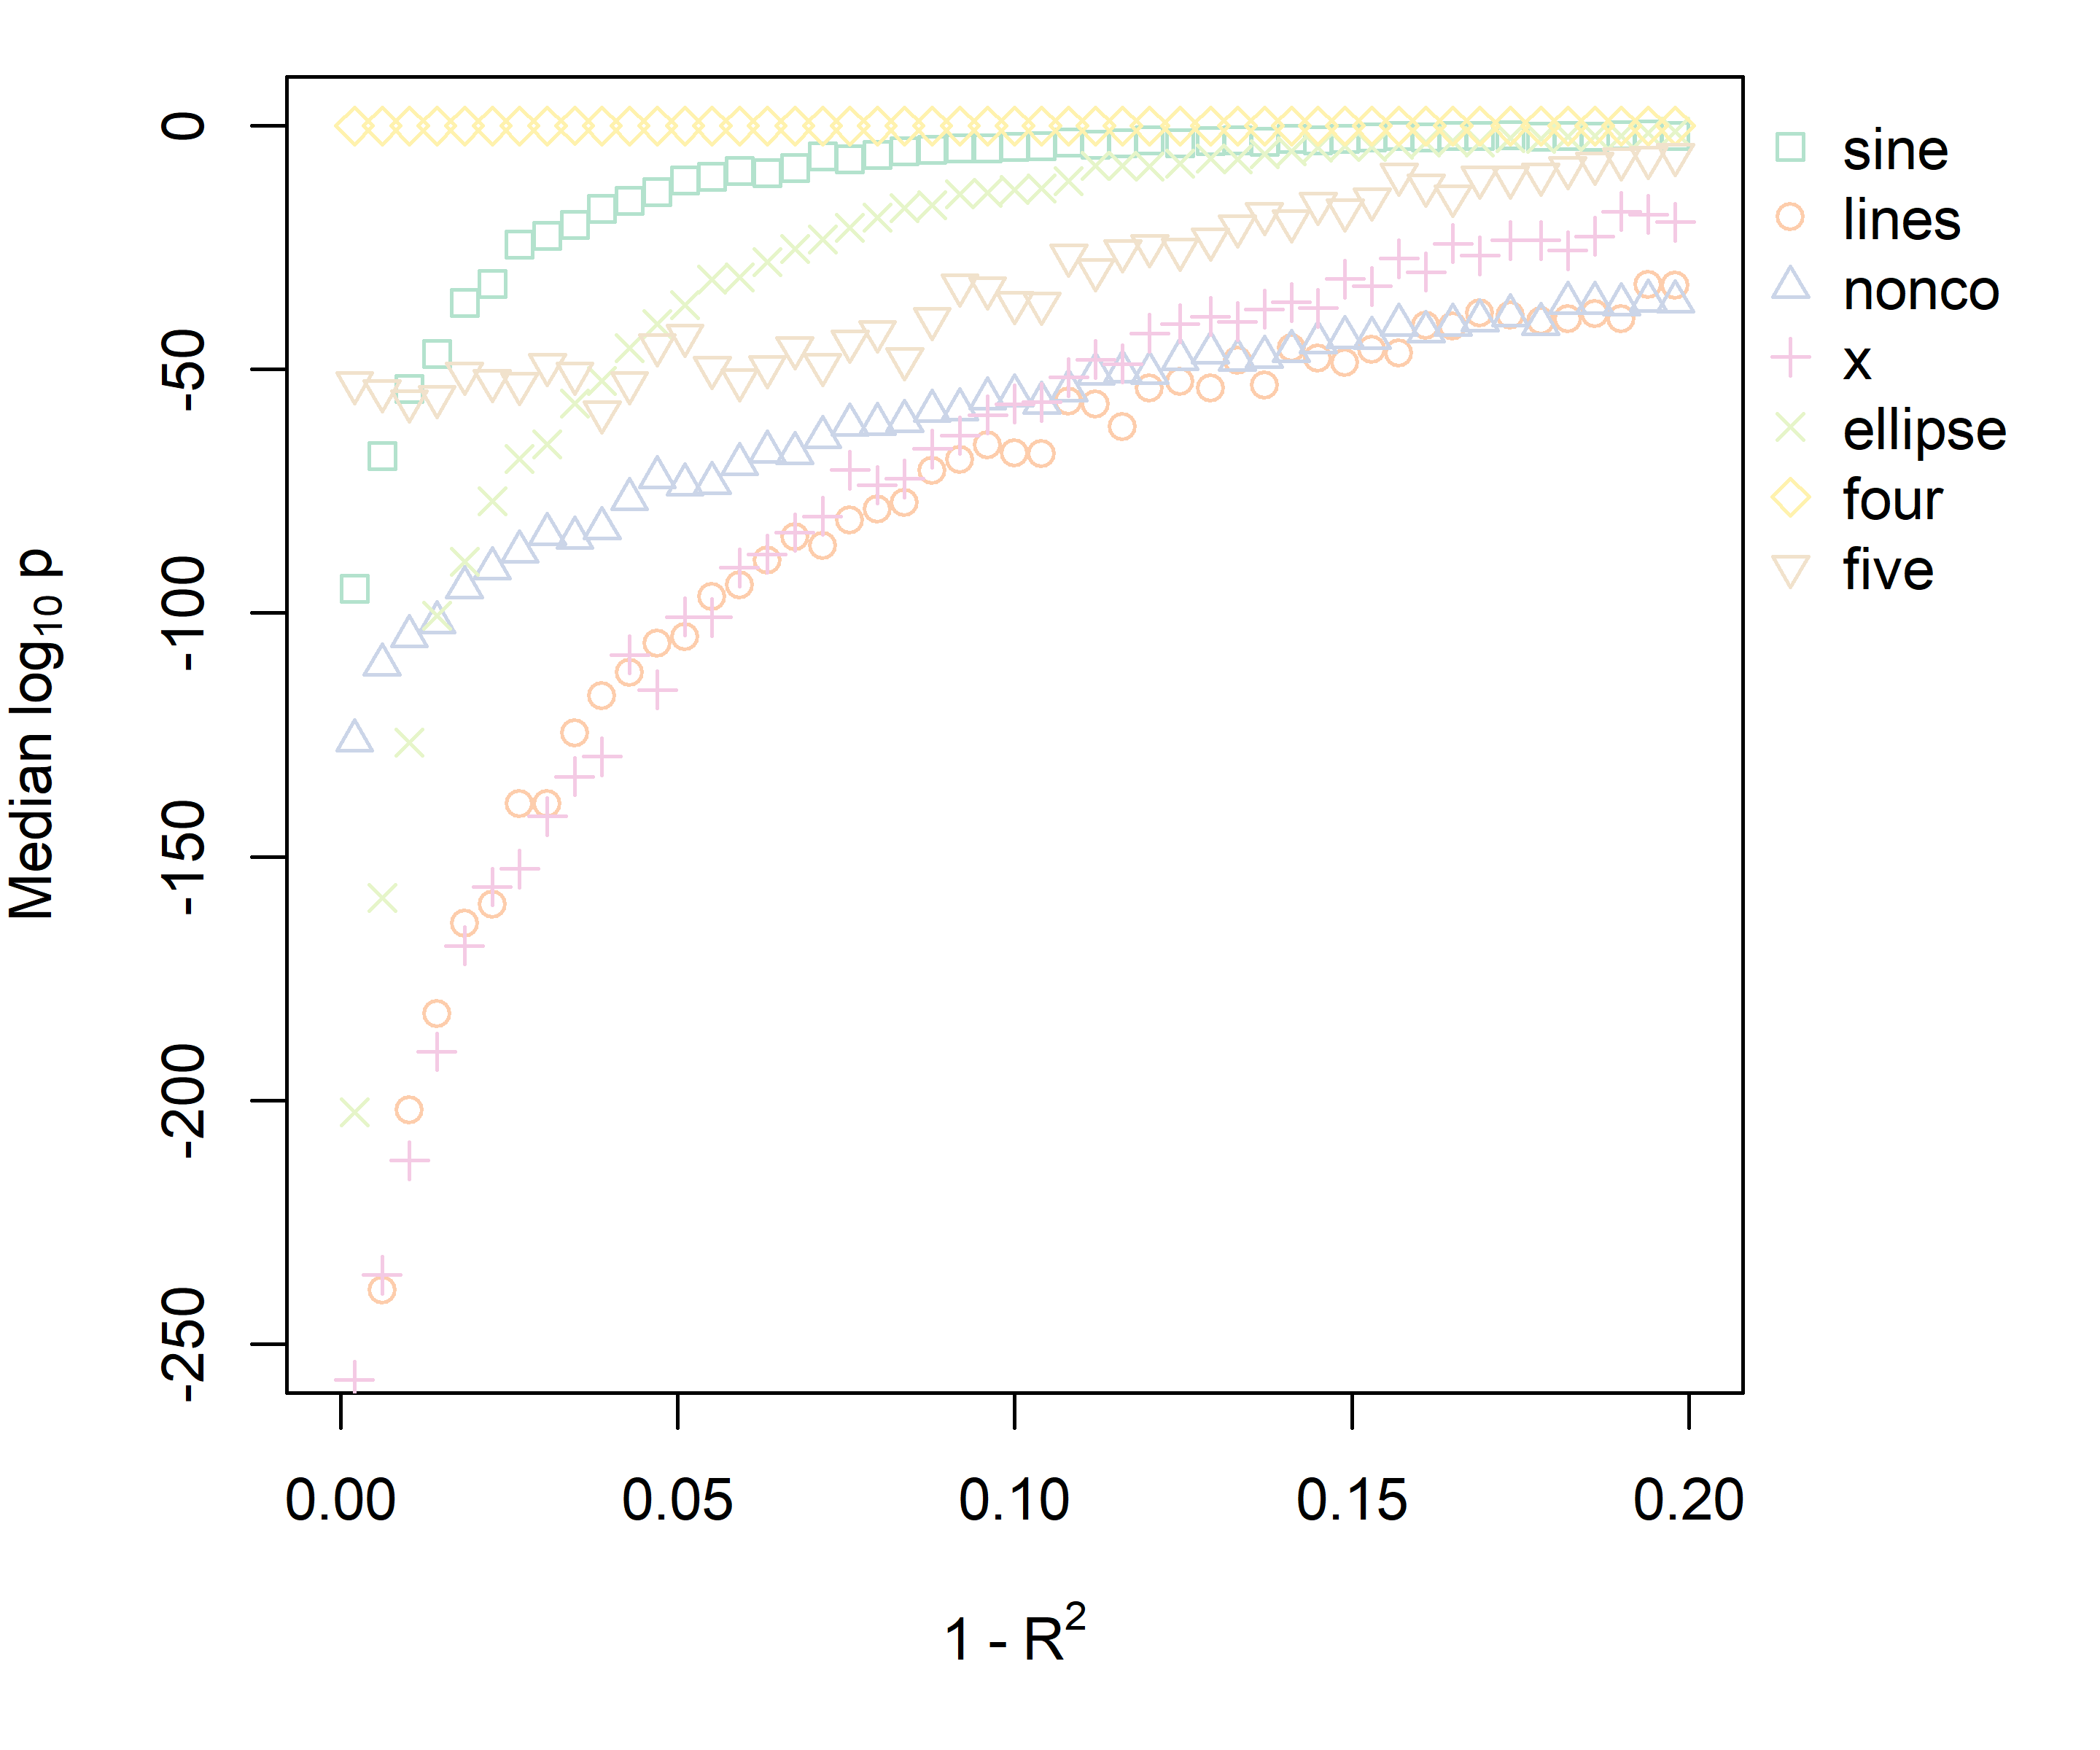}
			\vspace{-0.045\textheight}
	\caption{\footnotesize Zoom in on low noise -- median $\log_{10} p$}
	\label{fig:plotNoiseExamplePerfZoom}
	\end{subfigure}
	\end{tabular}
        \vspace{0.08\textheight}
			\caption{\footnotesize Independence testing by recursive random binning for fixed signals and various noise levels.  All non-noise patterns are dependent with the exception of the `four' pattern. 
			Each sample has 1000 points, the medians are based on 250 repeated samples. }
		\label{fig:plotNoiseExample}
	\end{center}
\end{figure}
For the same amount of added noise quantified by $R^2$ (pattern variance over pattern plus noise variance), the patterns do not display the same degree of dependence in their point clouds.
The line and non-coexistance patterns in the second and third row, for example, show clear distortions in their point clouds even when $R^2 = 0.5$ while the sine wave, ellipse, and pattern of five clusters seem scarcely different than random noise.
The ordering of $p$-values produced by $\bigChi$ and random recursive rank binning is consistent with this in Figures \ref{fig:plotNoiseExample}(b-c), and it is not obvious why this behaviour is undesirable.
